# Supplementary material for: Backpressure Flow Control
Source: arXiv:1909.09923 source file (2021-03-29)
Supplement: Supplementary file 1 [file appendix.tex]

\section{Deadlock prevention}
\label{app:deadlock}
We formally prove that BFC is deadlock-free in absence of cyclic buffer dependency. Inspired by Tagger~\cite{hu2017tagger}, we define a backpressure graph ($G(V, E)$) as follows:
\begin{enumerate}
    \item Node in the graph ($V$): A node in the graph is an egress port in a switch and can thus be represented by the pair <switchID, egressPort>. 
    \item Edge in the graph ($E$): There is a directed edge from $B \rightarrow A$, if a packet can go from $A$ to $B$ in a single hop (i.e., without traversing any other nodes) and trigger backpressure from $B \rightarrow A$. Edges represent how backpressure can propagate in the topology.
\end{enumerate}

We define deadlock as a situation when a node (egress port) contains a physical queue that has been paused indefinitely. Cyclic buffer dependency is formally defined as the situation when $G$ contains a cycle.

\begin{theorem}
BFC is deadlock-free if $G(V, E)$ does not contain any cycles.
\end{theorem}

\noindent\textit{Proof:} We prove the theorem by using contradiction. 

Consider a node $A$ that is deadlocked. $A$ must contain a physical queue ($A_q$) that has been indefinitely paused as a result of backpressure from the downstream switch. If all the packets sent by $A_q$ were drained from the downstream switch, then $A_q$ will get unpaused (\S\ref{s:backpressure}). Since BFC NICs don't generate backpressure, there must be atleast one node  ($B$) in the downstream switch that triggered backpressure to $A_q$ but hasn't been able to drain packets from $A_q$, i.e., $B$ is deadlocked. This implies, in $G$, there must be an edge from $B \rightarrow A$. Applying induction, for $B$ there must exist another node $C$ (at the downstream switch of $B$) that is also deadlocked (again there must be an edge from $C \rightarrow B$). Therefore, there will be an infinite chain of nodes which are paused indefinitely, the nodes of the chain must form a path in $G$. Since $G$ doesn't have any cycles, the paths in $G$ can only be of finite length, and therefore, the chain cannot be infinitely long. A contradiction! Hence proved.

\smallskip
\noindent\textbf{Preventing deadlocks:}
To prevent deadlocks, given a topology, we calculate the backpressure graph, and pre-compute the edges that should be removed so that the backpressure graph doesn't contain any cycles. Removing these edges, thus guarantees that there will be no deadlocks even under link failures or routing errors. To identify the set of edges that should be removed we can leverage existing work~\cite{hu2017tagger}.

To remove a backpressure edge $B \rightarrow A$, we use the simple strategy of skipping the backpressure operation for packets coming from $A$ going to $B$ at the switch corresponding to $B$\footnote{To remove backpressure edges in PFC, Tagger uses a more complex approach that invloves creating new cycle free backpressure edges corresponding to the backpressure edges that should be removed. To ensure losslessness, Tagger generates backpressure using these new cycle free edges instead of the original backpressure edge. In BFC, we forgo such requirement for simplicity.}. Note that, a switch can identify such packets \emph{locally} using the ingress and egress port of the packet. This information can be stored as a match-action-table (indexed by the ingress and egress port) to check whether we should execute the backpressure operations for the packet.

For clos topologies, this just includes backpressure edges corresponding to packets that are coming from a higher layer and going to higher layer (can happen due to rerouting in case of link failures). Note that, usually the fraction of such packets is small (< 0.002\%~\cite{hu2017tagger}), so forgoing backpressure for a small fraction of such packets, if at all should hurt performance only marginally. Having said that, in case the fraction is higher, we advocate running BFC with some form of end to end congestion control (\eg maintaining a cap on the in-flight packets) to avoid filling up the buffers.

\section{Incast flow performance}
\label{app:incast_fct}
\begin{figure}
    \centering
        \includegraphics[width=0.4\columnwidth]{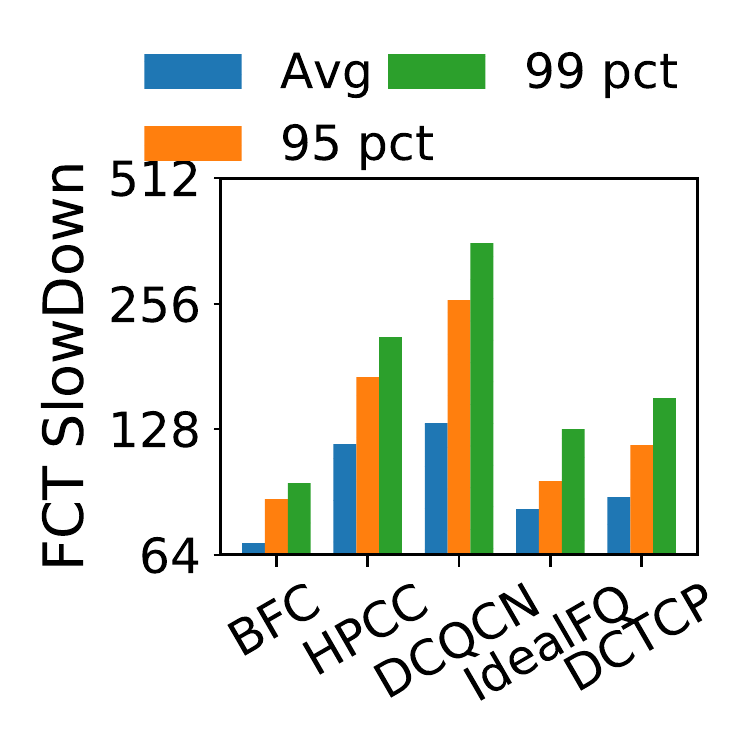}
        \vspace{-5mm}
        \caption{\small{FCT (incast).} BFC also reduces the FCT for incast flows compared to other schemes. Setup from \Fig{google_incast}.}
        \label{fig:google_incast:fct_incast}
\end{figure}

\Fig{google_incast:fct_incast} shows the slowdown for incast flows for the Google workload used in \Fig{google_incast}. BFC improves the performance of incast flows relative to end-to-end congestion control, as it maintains sufficient buffering to ensure incast packets are always in the queue.

\cut{
% moved figure back inline for now
\section{Impact of using slow start}
\label{app:ss}
  \begin{figure}[t]
    \centering
    \begin{subfigure}[tbh]{0.235\textwidth}
        \includegraphics[width=\textwidth]{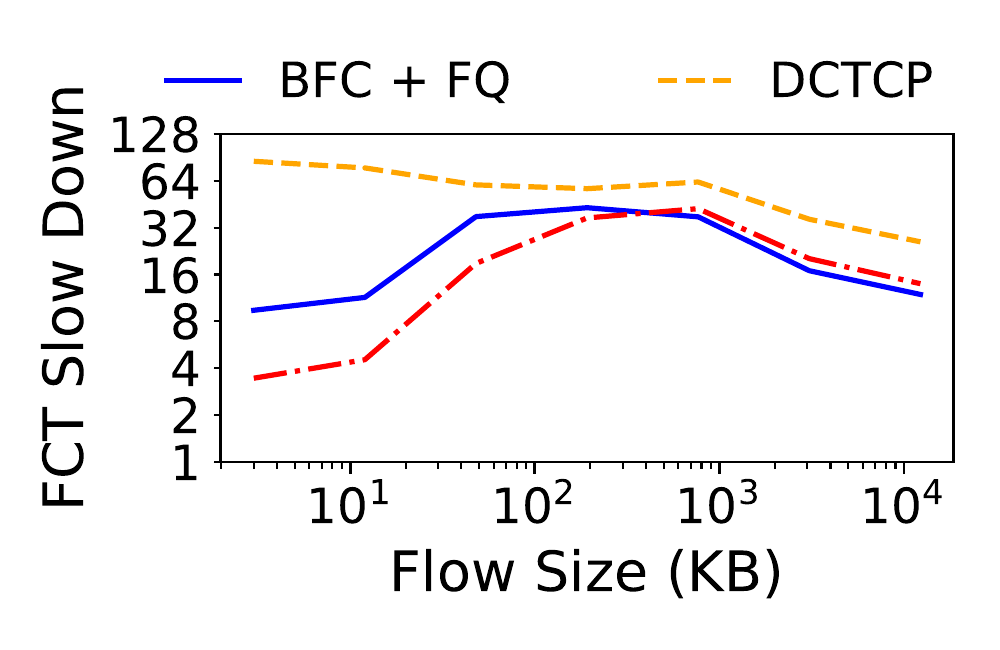}
        \vspace{-7mm}
        \caption{55\% + 5\% 100-1 incast}
        \label{fig:ss:incast}
    \end{subfigure}
    \begin{subfigure}[tbh]{0.235\textwidth}
        \includegraphics[width=\textwidth]{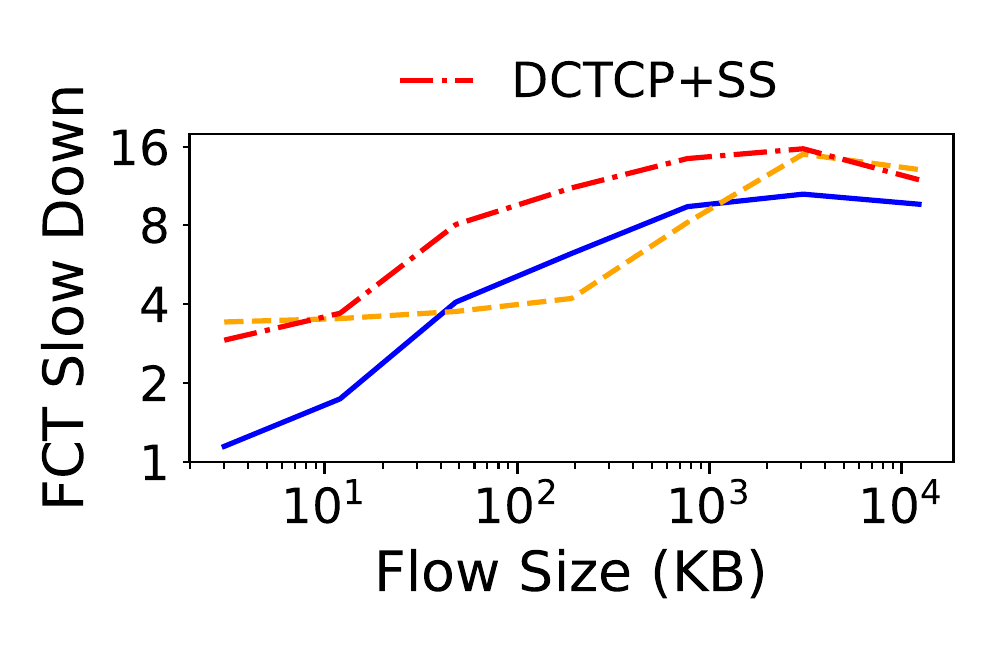}
        \vspace{-7mm}
        \caption{60\%}
        \label{fig:ss:no_incast}
    \end{subfigure}
    \vspace{-3mm}
    \caption{\small Impact of using slow start. DCTCP + SS (slow start) reduces FCTs in the presence of incast. However, in the absence of incast, it increases the FCT for medium flows.}
    \label{fig:ss}
    \vspace{-4mm}
\end{figure}
We compare the original DCTCP with slow start (DCTCP + SS) and our modified DCTCP used so far (i.e., flows start at the line rate), the setup is same as \Fig{fb_variants}. \Fig{ss} shows the 99$^{th}$ percentile FCT slowdown. We used an initial congestion window of 10 for DCTCP + SS. A DCTCP + SS flow starts at a rate lower than the line rate, and can have atmost 10 packets in flight in the first RTT. In contrast, a DCTCP flow can have upto 1-BDP (or 100 packets) in flight in the first RTT. As a result, with incast, DCTCP + SS significantly reduces buffer occupancy and PFC triggers caused by the sudden arrival of incast flows, and the FCTs are better compared to DCTCP. However, DCTCP + SS increases the FCTs for medium flows (0.5-5 BDP) in the absence of incast. With DCTCP + SS, a flow starts at a lower rate, it can take multiple RTTs to ramp up to the desired rate, hurting latency. Using slow-start thus presents a trade-off. In contrast, with BFC there is no such trade-off, all flows can start directly at the line rate as buffers are better managed using per-hop control.
}

\section{Impact of spatial locality}
\label{app:load_var:locality}
 
 \begin{figure}[t]
    \centering
    \begin{subfigure}[tbh]{0.235\textwidth}
        \includegraphics[width=\textwidth]{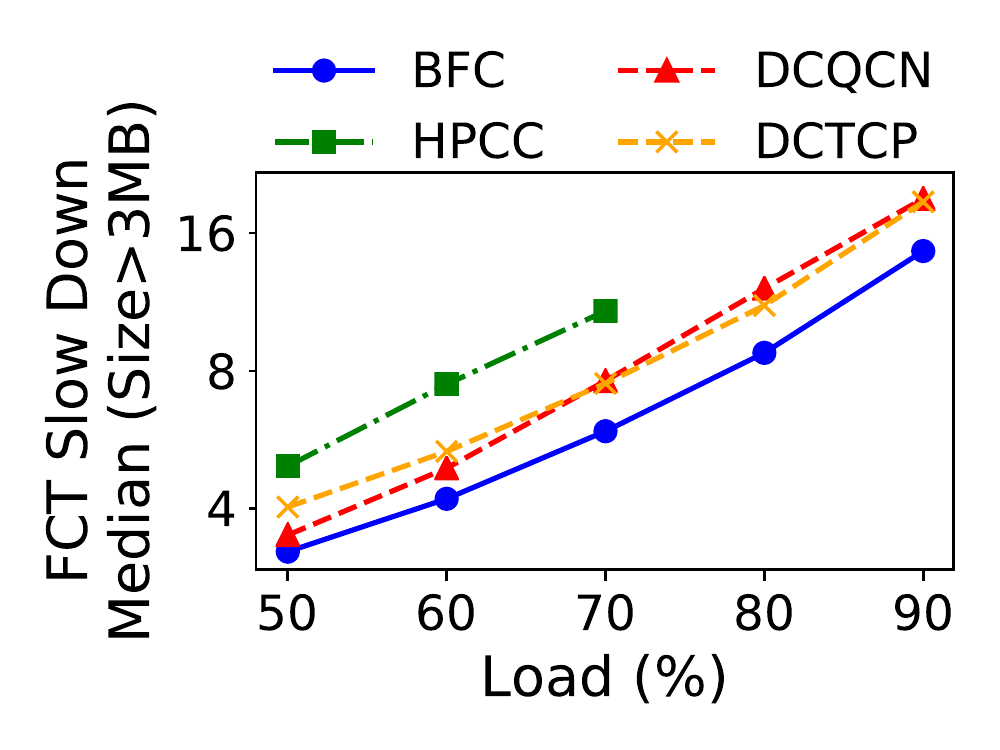}
         \vspace{-7mm}
        \label{fig:load_var_locality:long}
        \caption{FCT for long flows}
    \end{subfigure}
    \begin{subfigure}[tbh]{0.235\textwidth}
        \includegraphics[width=\textwidth]{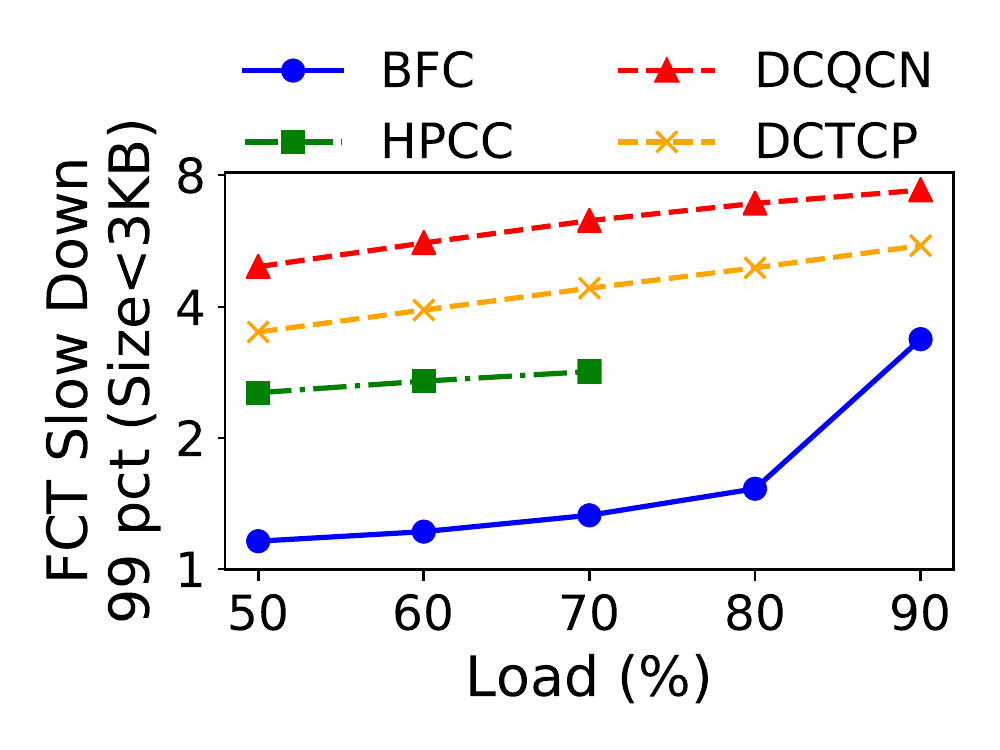}
        \vspace{-7mm}
        \caption{FCT for short flows}
        \label{fig:load_var_locality:small}
        
    \end{subfigure}
    \vspace{-3mm}
    \caption{\small Impact of traffic load on performance with spatial locality.}
    \label{fig:load_var_locality}
    \vspace{-5mm}
\end{figure}
We repeated the experiment from \Fig{load_var} with spacial locality in source-destination pairs such that the average load on all links across the network is same. \Fig{load_var_locality} show the slowdowns. The trends are similar to \Fig{load_var}. In particular, the FCT slowdowns for BFC are very similar with and withouy locality. For long flows, the performance for HPCC and DCQCN improves compared to that in \Fig{load_var}. With locality, 50\% of the flows are within the same ToR, the RTT for such flows is smaller (4us). With smaller RTTs, these protocols react much faster improving FCT slowdown for intra-rack flows, and driving down the overall median FCTs.

\section{Sensitivity to resource constraints}
\label{app:sensitivity}

\smallskip
\noindent\textbf{Number of FIDs:} 
\begin{figure}[t]
    \centering
    \begin{subfigure}[t]{0.45\textwidth}
        \includegraphics[width=\textwidth]{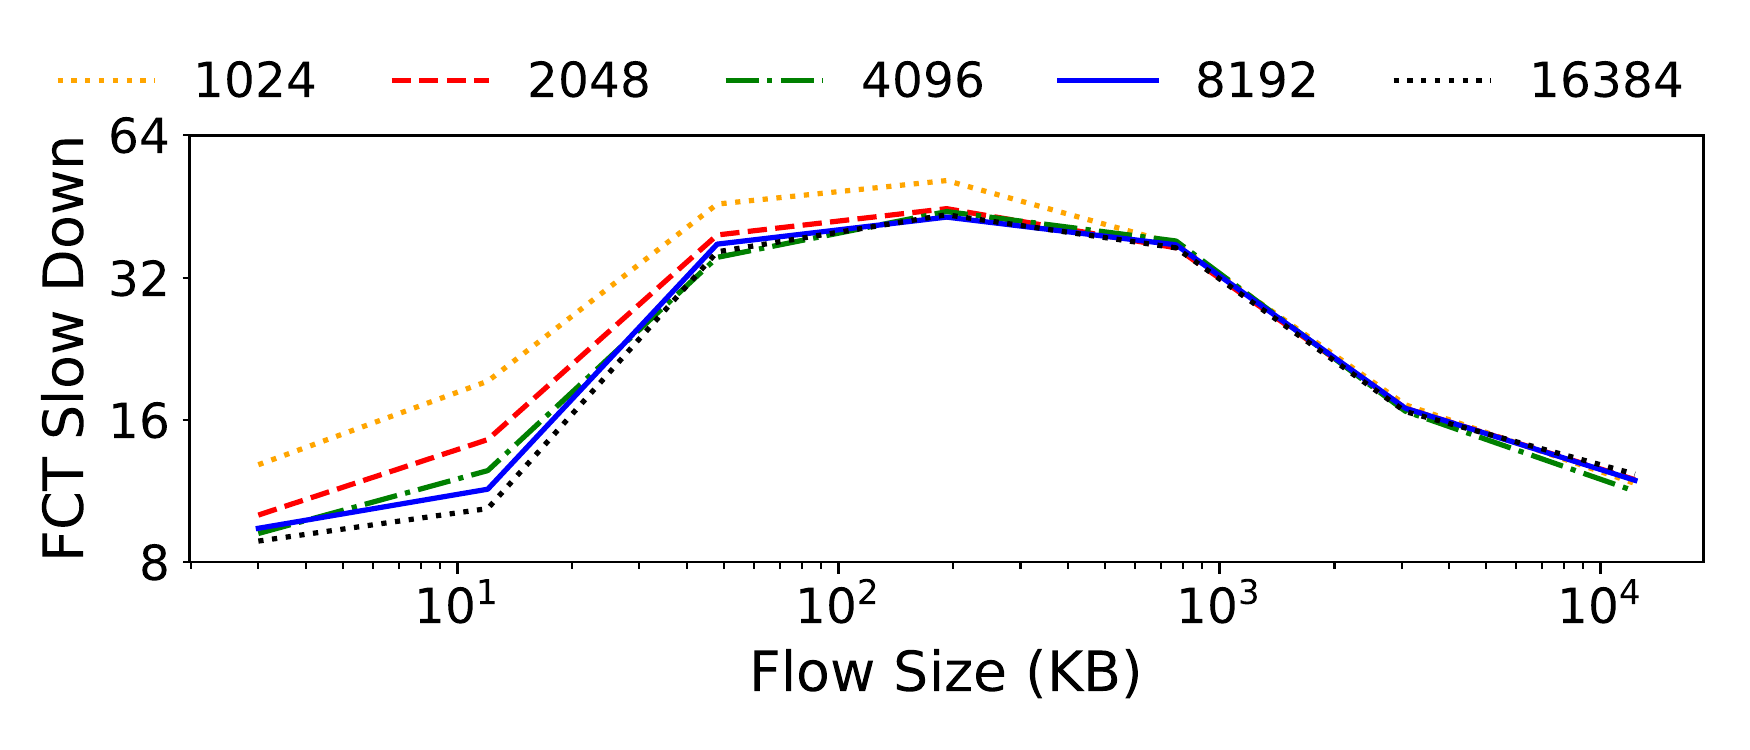}
        \vspace{-6mm}
        \caption{99$^{th}$ percentile FCT}
        \label{fig:impact_vq:fct}
    \end{subfigure}
    \vspace{-3mm}
    \caption{\small Tail latency as a function of the size of the flow hash table (number of buckets). 
    Reducing the size of the flow table but has limited effect on performance.}
    \label{fig:impact_vq}
    \vspace{-5mm}
\end{figure}
We repeated the experiment from \Fig{pq:incast}, but varied the size of the flow hash table. \Fig{impact_vq:fct} shows the tail latency across different scenarios. On this workload,
\bfc{}'s performance is not sensitive to the size of the flow hash table. 
Tail latencies degrade marginally when the number of buckets is reduced to 1024.
This might allow the switch to use a smaller hash table, but we note that other
workloads, such as those with higher utilization and smaller flows, may be more
sensitive to the hash table size.

%The number of collisions and overflows are less than 1.5\% in all the cases.
